# Supplementary material for: Disorder-induced symmetry breaking in moir\'e bands of marginally twisted bilayer MoS$_2$
Source: arXiv:2602.06318 ancillary file (2026-02-06)
Supplement: Supplementary file 1 [file Supporting_information.pdf]

# SUPPORTING INFORMATION
# Disorder-induced symmetry breaking in moiré bands of marginally twisted bilayer $MoS_2$

Pablo Reséndiz-Vázquez,[1] Christophe de Beule,[2,3] Thi-Hai-Yen Vu,[1] Kaijian Xing,[1] Daniel McEwen,[1] Daniel Bennett,[4,5] Liangtao Peng,[6] Héctor González-Herrero,[7,8] Shaffique Adam,[6] Mark T. Edmonds,[1] and Michael S. Fuhrer[1]

[1]*School of Physics and Astronomy, Monash University, Clayton, Victoria 3800, Australia*
[2]*Department of Physics and Astronomy, University of Pennsylvania, Philadelphia, Pennsylvania 19104, USA*
[3]*Department of Physics, University of Antwerp, Groenenborgerlaan 171, 2020 Antwerp, Belgium*
[4]*John A. Paulson School of Engineering and Applied Sciences, Harvard University, Cambridge, Massachusetts 02138, USA*
[5]*School of Electrical and Electronic Engineering, Nanyang Technological University Singapore, 50 Nanyang Avenue, 639798, Singapore*
[6]*Department of Physics, Washington University, St. Louis, Missouri 63130, USA*
[7]*Departamento de Física de la Materia Condensada, Universidad Autónoma de Madrid, E-28049 Madrid, Spain*
[8]*Condensed Matter Physics Center (IFIMAC), Universidad Autónoma de Madrid, E-28049, Madrid, Spain*

## S1. SAMPLE DETAILS

Fig. S1 presents the studied sample and all its components. Fig. S1a is an optical image of the device before transferring to the STM chamber. The color code follows the schematic presented in Fig. S1b, where a side view of the device is shown. The metallic contact was deposited by electron beam physical vapour deposition and have a composition of 10 nm of Chromium followed by 10 nm of Platinum on top. The graphite flake has an approximate thickness of 30 nm, based on a color contrast scale confirmed by atomic force microscopy.

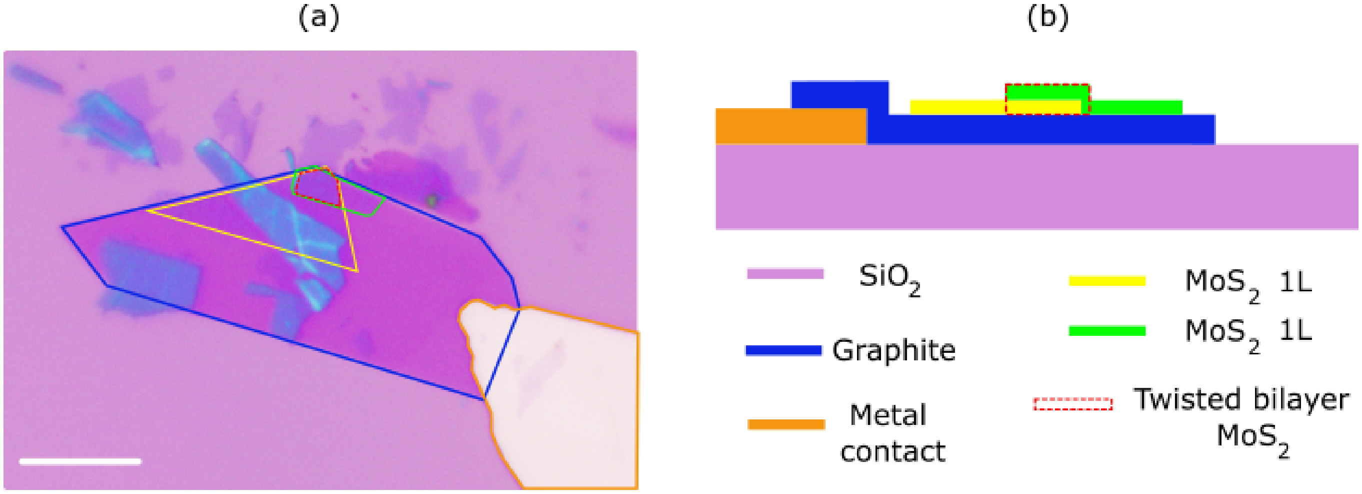


FIG. S1. Twisted bilayer $MoS_2$ sample. (a) Optical micrograph of the sample, the metallic electrode supplies contact to the graphite and a visual guide for navigation. Scale bar is 10 $\mu$m. (b) Side-view schematic of the sample composition. $MoS_2$ 1L refers to monolayer $MoS_2$.

## S2. ONSET BIAS CALCULATION

Fig. S2 illustrates the method to obtain the bias value at the band edge. It is determined as the intersection of a linear fit along the edges (green lines) of the log(dI/dV) curve with an arbitrary noise floor at $2.5 \times 10^{-2}$ (arb. units) (red dashed line). In this case these intersections are the red and blue dots, respectively. The onset is the bias value at which these intersections occur (gray dashed lines).

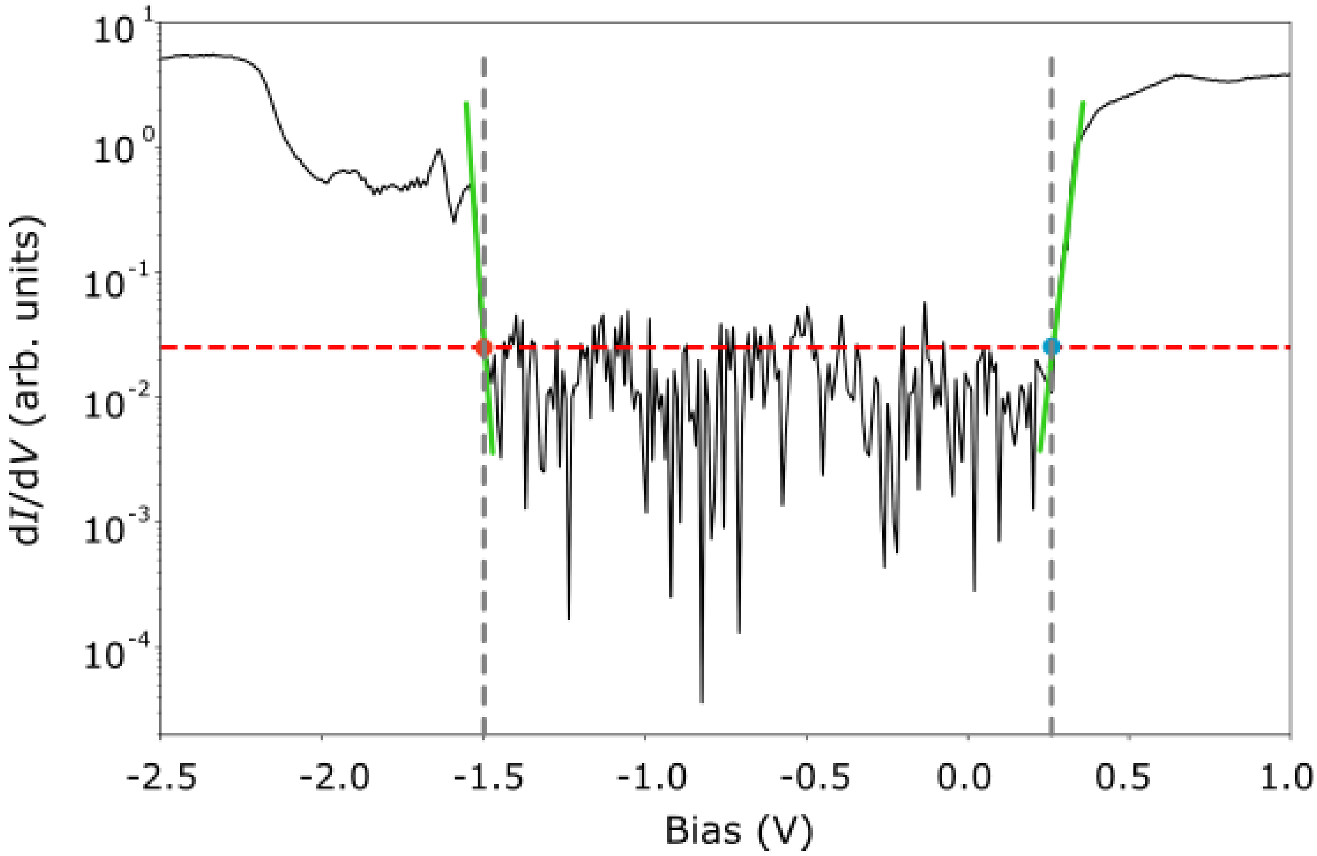


FIG. S2. Determining the onset bias values. Example of a point STS around the band gap. Parameters: $V_{\text{bias}} = -2.5$ V, $I_{\text{set}} = 250$ pA. The vertical axis of the plot is in logarithmic scale.

## S3. ELECTRONIC THEORY

### A. Untwisted bilayers

We start with a model near the top of the valence band or bottom of the conduction band of untwisted aligned bilayer 2H $MoS_2$ (3R stacking). To this end, we construct an effective Hamiltonian near $\Gamma$ or $K/K'$ as a function of the interlayer stacking vector $\boldsymbol{\phi}$. In layer basis, this Hamiltonian can be written as

$$H_Q(\boldsymbol{k}, \boldsymbol{\phi}) = \begin{bmatrix} \frac{\hbar^2 k^2}{2m_Q} + \epsilon_Q(\boldsymbol{\phi}) & t_Q(-\boldsymbol{\phi}) \\ t_Q(\boldsymbol{\phi}) & \frac{\hbar^2 k^2}{2m_Q} + \epsilon_Q(-\boldsymbol{\phi}) \end{bmatrix}, \tag{S1}$$

where $\boldsymbol{k} = (k_x, k_y)$ is the Bloch momentum, $m_Q$ is the effective mass at valley $Q$, and $\boldsymbol{\phi} = (\phi_x, \phi_y)$ is the interlayer disregistry. For example, $\boldsymbol{\phi} = (0, 0)$ corresponds to MM stacking while $\boldsymbol{\phi} = (0, \pm a/\sqrt{3})$ is MX/XM stacking with $a$ the lattice constant. Here we choose coordinates such that the zigzag direction of the monolayer lies along the $x$ axis. Moreover, we only consider the $\Gamma$ and $K/K'$ point such that the effective mass is isotropic due to threefold rotation symmetry. An example of the band structure obtained from density functional theory (DFT) calculations is shown in Fig. S3 for two stacking configurations with an without spin-orbit coupling (SOC). In Eq. (S1) we already used that the 2H $MoS_2$ bilayers have a mirror symmetry about the plane ($z \mapsto -z$),

$$H_Q(\boldsymbol{k}, \boldsymbol{\phi}) = \sigma_x H_Q(\boldsymbol{k}, -\boldsymbol{\phi}) \sigma_x, \tag{S2}$$

where $\sigma_x$ is a Pauli matrix that acts on layer space. Here we used that a layer reversal is equivalent to changing the sign of the interlayer shift. This will turn out to only be an approximate symmetry of the moiré theory. Furthermore, periodicity of the monolayer implies

$$H_Q(\boldsymbol{k}, \boldsymbol{\phi} + \boldsymbol{a}) = H_Q(\boldsymbol{k}, \boldsymbol{\phi}), \tag{S3}$$

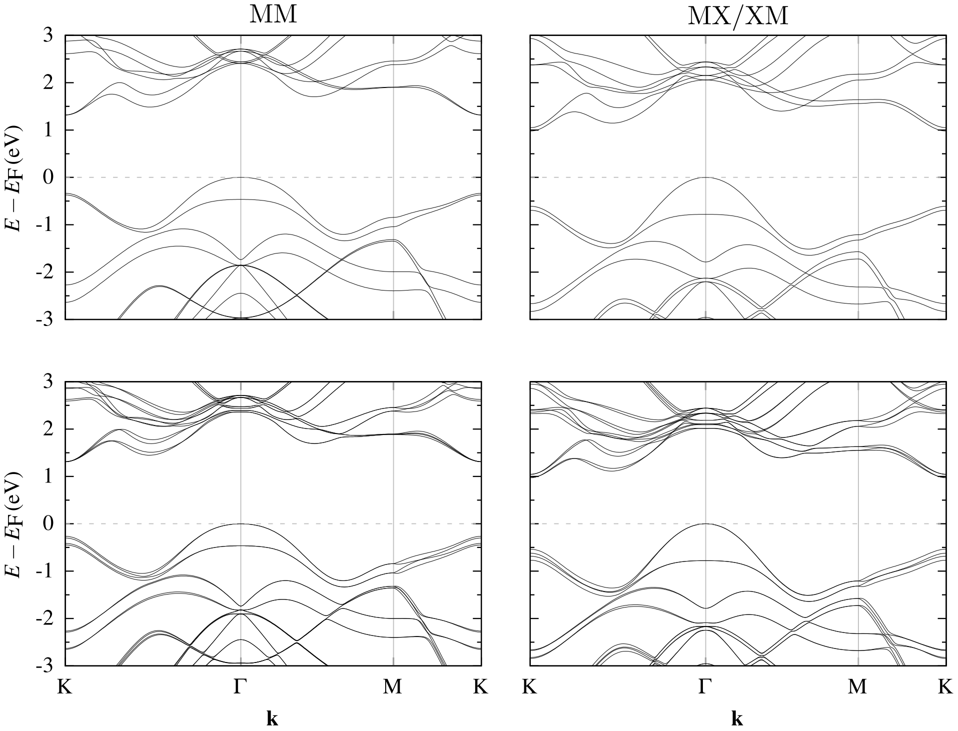


FIG. S3. Band structure of untwisted aligned 2H $MoS_2$ bilayers for two high-symmetry stacking configurations. Calculated using DFT without (top) and with (bottom) SOC.

where $\boldsymbol{a}$ is a monolayer lattice vector. Above we also defined the intralayer potential $\epsilon(\boldsymbol{\phi})$ and the interlayer tunneling amplitude $t(\boldsymbol{\phi})$.

### B. Symmetry constraints

The functions $\epsilon(\boldsymbol{\phi})$ and $t(\boldsymbol{\phi})$ can be further constrained by the symmetries of the monolayer. The point group of a transition metal dichalcogenide (TMD) monolayer in the trigonal prismatic (2H) phase is given by $D_{3h} = D_3 \times \sigma_h = C_{3v} \times \sigma_h$ with $D_3 = \langle \mathcal{C}_{3z}, \mathcal{C}_{2y} \rangle$. Here $\mathcal{C}_{3z}$ is a threefold rotation about the $z$ axis and $\mathcal{C}_{2y}$ is twofold rotation about the $y$ axis. These symmetries yield

$$\begin{aligned} H_Q(\boldsymbol{k}, \mathcal{C}_{3z}\boldsymbol{\phi}) &= H_{\mathcal{C}_{3z}Q}(\mathcal{C}_{3z}\boldsymbol{k}, \boldsymbol{\phi}) \\ H_Q(\boldsymbol{k}, \mathcal{C}_{2y}\boldsymbol{\phi}) &= \sigma_x H_{\mathcal{C}_{2y}Q}(-k_x, k_y, \boldsymbol{\phi})\sigma_x \\ &= H_{\mathcal{C}_{2y}Q}(-k_x, k_y, -\boldsymbol{\phi}), \end{aligned} \tag{S4}$$

where the last line follows from Eq. (S2). In our case, we only consider the $\Gamma$ and $K/K'$ valleys such that $\mathcal{C}_{3z}Q = Q + b$ and we choose $\mathcal{C}_{2y}Q = -Q$. However, since the two layers are separated by $\boldsymbol{\phi}$ which is generally not a lattice vector, the Bloch wave function picks up a relative phase:

$$H_{\mathcal{C}_{3z}Q} = H_{Q+(\mathcal{C}_{3z}Q-Q)} = U_Q H_Q U_Q^\dagger, \tag{S5}$$

where $U_Q$ is a diagonal phase matrix. We have $U_\Gamma = \mathbb{1}_2$ and $U_K = U_{K'}^* = e^{i\sigma_z(\boldsymbol{b}_1+\boldsymbol{b}_2)\cdot\boldsymbol{\phi}/2}$. Moreover, since $Q$ and $-Q$ are related by time-reversal symmetry, we have

$$\begin{aligned} H_Q(\boldsymbol{k}, \boldsymbol{\phi}) &= [H_{-Q}(-\boldsymbol{k}, \boldsymbol{\phi})]^* \\ &= [H_Q(-k_x, k_y, -\phi_x, \phi_y)]^* . \end{aligned} \tag{S6}$$

We then obtain the following conditions

$$\begin{aligned} \epsilon_Q(\boldsymbol{\phi}) &= \epsilon_Q(-\phi_x, \phi_y) = \epsilon_Q(\mathcal{C}_{3z}^{-1}\boldsymbol{\phi}), \\ t_Q(\boldsymbol{\phi}) &= t_Q^*(-\boldsymbol{\phi}) = t_Q(\phi_x, -\phi_y) \\ &= e^{i(\mathcal{C}_{3z}\boldsymbol{Q}-\boldsymbol{Q})\cdot\boldsymbol{\phi}} t_Q(\mathcal{C}_{3z}^{-1}\boldsymbol{\phi}). \end{aligned} \tag{S7}$$

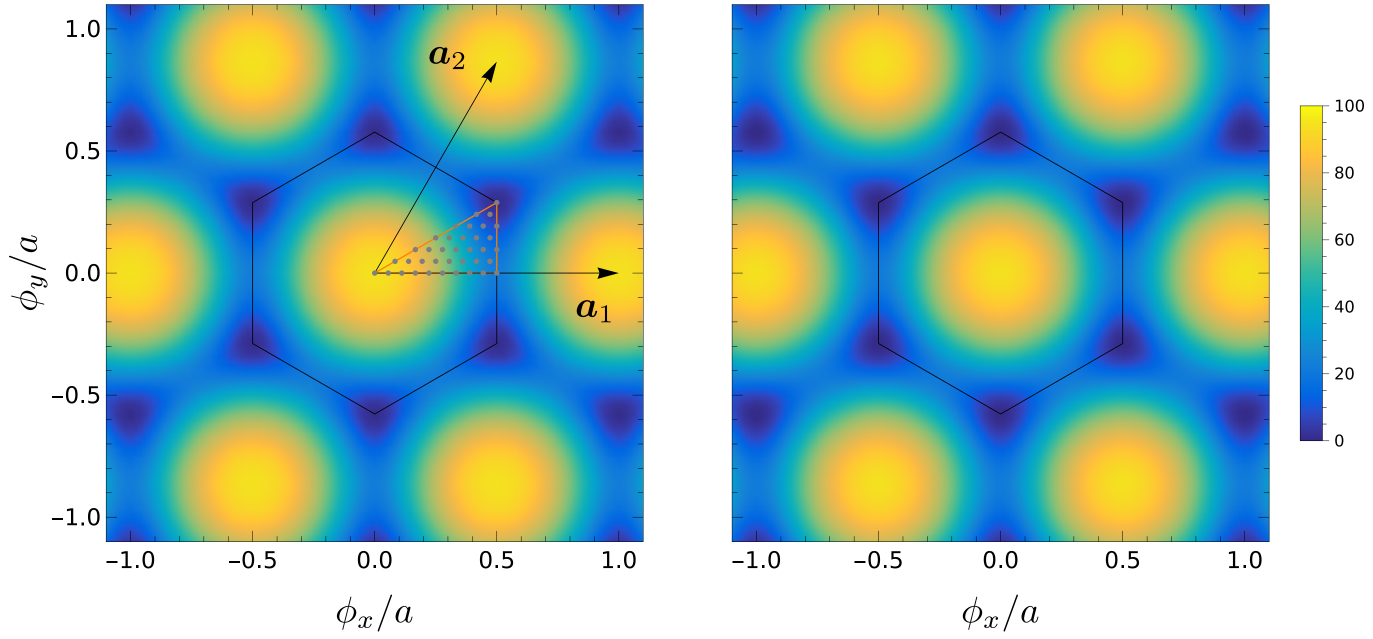


FIG. S4. Adhesion energy in units of meV per monolayer unit cell relative to the lowest-energy configuration for (untwisted) aligned 2H $MoS_2$ bilayers as a function of the stacking configuration $\boldsymbol{\phi} = (\phi_x, \phi_y)$ in units of the monolayer lattice constant $a$. Here the origin corresponds to MM stacking and the corners of the hexagon to MX/XM stacking. (left) Interpolated adhesion potential using 37 DFT data points shown as the gray dots. The orange triangle contains all configurations that are not related by symmetry. (right) Fit of the adhesion potential obtained by numerically computing the inverse Fourier transform of the data shown in the left panel.

The last equations imply that $t_Q(\boldsymbol{\phi})$ is real for $\boldsymbol{\phi} = \boldsymbol{a}/2$ which corresponds to MM and DW stacking. Furthermore, we have

$$\left(1 - e^{i\boldsymbol{Q}\cdot\boldsymbol{a}}\right) t_Q(\boldsymbol{\phi}) = 0 \quad \text{for} \quad \mathcal{C}_{3z}^{-1}\boldsymbol{\phi} = \boldsymbol{\phi} + \boldsymbol{a}, \tag{S8}$$

such that $t_{K/K'}$ vanishes for MX/XM stacking.

Since the intralayer potential has to be real, we have the Fourier expansion

$$\begin{aligned} \epsilon_Q(\boldsymbol{\phi}) = V_0 &+ 2V_1 \sum_{n=1}^{3} \cos(\boldsymbol{b}_n \cdot \boldsymbol{\phi} + \psi_1) \\ &+ 2V_2 \sum_{n=1}^{3} \cos(\boldsymbol{b}'_n \cdot \boldsymbol{\phi}) \\ &+ 2V_3 \sum_{n=1}^{3} \cos(2\boldsymbol{b}_n \cdot \boldsymbol{\phi} + \psi_3) \\ &+ \cdots , \end{aligned} \tag{S9}$$

where $\boldsymbol{b}_n$ ($\boldsymbol{b}'_n$) are reciprocal lattice vectors of the monolayer that belong to the first (second) star and which are related by $\mathcal{C}_{3z}$ rotations. We take $\boldsymbol{b}_1 = 4\pi\hat{y}/\sqrt{3}a$, $\boldsymbol{b}_2 = \mathcal{C}_{3z}\boldsymbol{b}_1$, and $\boldsymbol{b}'_1 = \boldsymbol{b}_1 - \boldsymbol{b}_2$. Note that $\psi_2 = 0$ because of the first equality in Eq. (S7). Here we also choose $V_0 = 0$ and take $V_{1,3} > 0$ for convenience. To keep the notation simple, we did not explicitly denote the dependence of the coefficients $V_i$ ($i = 1, 2, 3$) on valley $Q$.

### $\Gamma_v$ *valley*

At the $\Gamma$ point, we have time-reversal symmetry. Moreover, we find that the states at the valence band maximum originate mostly from metal $d_z^2$ and chalcogen $p_z$ orbitals such that SOC vanishes, as can be seen in Fig. S3. Hence

the Hamiltonian is real and spin degenerate at $\Gamma_v$. Therefore, we have

$$\begin{aligned} t_\Gamma(\boldsymbol{\phi}) = t_\Gamma(-\boldsymbol{\phi}) = w_0 &+ 2w_1 \sum_{i=1}^{3} \cos(\boldsymbol{b}_i \cdot \boldsymbol{\phi}) \\ &+ 2w_2 \sum_{i=1}^{3} \cos(\boldsymbol{b}'_i \cdot \boldsymbol{\phi}) \\ &+ 2w_3 \sum_{i=1}^{3} \cos(2\boldsymbol{b}_i \cdot \boldsymbol{\phi}) \\ &+ \cdots . \end{aligned} \tag{S10}$$

*$K_c/K'_c$ valley*

From the DFT results, we observe that the bottom of the conduction band is at $K/K'$ and that SOC is almost negligible. Here we find that the states originate mostly from metal $d_{z^2}$ orbitals with small contributions from chalcogen $p_{x,y}$ orbitals. Hence there is also an approximate spin degeneracy. However, unlike for the $\Gamma$ valley, the models at $K$ and $K'$ are related by time-reversal symmetry such that $t(\boldsymbol{\phi})$ can be complex. Taking $\boldsymbol{K} = -(\boldsymbol{b}_1 + 2\boldsymbol{b}_2)/3 = 4\pi\hat{x}/(\sqrt{3}a)$, the symmetry constraints yield

$$\begin{aligned} t_K(\boldsymbol{\phi}) = w_1 &\left(1 + e^{i\boldsymbol{b}_2\cdot\boldsymbol{\phi}} + e^{i(\boldsymbol{b}_1+\boldsymbol{b}_2)\cdot\boldsymbol{\phi}}\right) \\ &+ w_2 \left(e^{i\boldsymbol{b}_1\cdot\boldsymbol{\phi}} + e^{-i\boldsymbol{b}_1\cdot\boldsymbol{\phi}} + e^{i(\boldsymbol{b}_1+2\boldsymbol{b}_2)\cdot\boldsymbol{\phi}}\right) \\ &+ w_3 \left(e^{-i\boldsymbol{b}_2\cdot\boldsymbol{\phi}} + e^{-i(\boldsymbol{b}_1+\boldsymbol{b}_2)\cdot\boldsymbol{\phi}} + e^{2i(\boldsymbol{b}_1+\boldsymbol{b}_2)\cdot\boldsymbol{\phi}} + e^{i(2\boldsymbol{b}_1+\boldsymbol{b}_2)\cdot\boldsymbol{\phi}} + e^{2i\boldsymbol{b}_2\cdot\boldsymbol{\phi}} + e^{i(\boldsymbol{b}_2-\boldsymbol{b}_1)\cdot\boldsymbol{\phi}}\right) \\ &+ \cdots , \end{aligned} \tag{S11}$$

where all coefficients $w_i$ $(i = 1, 2, 3)$ are real.

*Fitting to DFT*

The two-band effective Hamiltonian for valley $Q$ can be written in layer basis as

$$H_Q(\boldsymbol{k}, \boldsymbol{\phi}) = \left[\frac{\hbar^2 k^2}{2m_Q} + \frac{\epsilon_Q(\boldsymbol{\phi}) + \epsilon_Q(-\boldsymbol{\phi})}{2}\right] \sigma_0 + \boldsymbol{d}_Q(\boldsymbol{\phi}) \cdot \boldsymbol{\sigma}, \tag{S12}$$

with $\boldsymbol{\sigma} = (\sigma_x, \sigma_y, \sigma_z)$ the three Pauli matrices that correspond here to the layer degree of freedom, and

$$\boldsymbol{d}_Q(\boldsymbol{\phi}) = \begin{pmatrix} \frac{t_Q(\boldsymbol{\phi})+t_Q(-\boldsymbol{\phi})}{2} \\ \frac{t_Q(\boldsymbol{\phi})-t_Q(-\boldsymbol{\phi})}{2i} \\ \frac{\epsilon_Q(\boldsymbol{\phi})-\epsilon_Q(-\boldsymbol{\phi})}{2} \end{pmatrix}. \tag{S13}$$

The energies are given by

$$E_{Q,\pm}(\boldsymbol{k}, \boldsymbol{\phi}) = \frac{\hbar^2 k^2}{2m_Q} + \frac{\epsilon_Q(\boldsymbol{\phi}) + \epsilon_Q(-\boldsymbol{\phi})}{2} \pm |\boldsymbol{d}_Q(\boldsymbol{\phi})|. \tag{S14}$$

The model parameters, namely coefficients of $\epsilon_Q(\boldsymbol{\phi})$ and $t_Q(\boldsymbol{\phi})$, were obtained by fitting to the band structures of the commensurate bilayer as a function of stacking, calculated using DFT (see Methods section of the main text). To sample the different possible local environments, we used 37 stacking configurations that are not related by symmetry on a triangular grid (see Fig. S4), which is compatible with the $C_{6v}$ symmetry of the adhesion potential. The results are shown in Table S1 for the $\Gamma_v$ and $K_c/K'_c$ point. We also calculate the effective mass of monolayer $MoS_2$ from the curvature of the valence and conduction bands about $\Gamma$ and K, respectively.

| $a$ (Å) | $m_{\Gamma_v}/m_e$ | $V_1$ | $V_2$ | $V_3$ | $\psi_1$ | $\psi_3$ | $w_0$ | $w_1$ | $w_2$ | $w_3$ |
|---|---|---|---|---|---|---|---|---|---|---|
| 3.1852 | −0.9 | 28.78 | 4.00 | 7.73 | 124.3° | −75.2° | 310.88 | −16.33 | 1.09 | 3.03 |

| $m_{K_c}/m_e$ | $V_1$ | $V_2$ | $V_3$ | $\psi_1$ | $\psi_3$ | $w_1$ | $w_2$ | $w_3$ |
|---|---|---|---|---|---|---|---|---|
| 0.5 | 5.67 | −0.17 | 1.16 | 80.0° | −97.8° | 1.06 | −0.45 | −0.05 |

TABLE S1. Fitting parameters for the effective Hamiltonian near the (top) $\Gamma_v$ and (bottom) $K_c/K_c'$ point of untwisted 2H $MoS_2$ bilayers. We also give the monolayer effective mass and lattice constant $a$. Energies are in units of meV.

### C. Local-stacking approximation

For small twist angles, such as those relevant to this work, the moiré pattern varies slowly on the interatomic scale, and one can describe the moiré in the long-wavelength limit with the local stacking configuration

$$\begin{aligned}\boldsymbol{\phi}(\boldsymbol{r}) &= R(\theta/2)\boldsymbol{r} - R(-\theta/2)\boldsymbol{r} + \boldsymbol{u}(\boldsymbol{r}) \\ &= \frac{a}{L}\hat{z}\times\boldsymbol{r} + \boldsymbol{u}(\boldsymbol{r}),\end{aligned} \tag{S15}$$

with $R(\theta)$ the rotation matrix for a counterclockwise rotation over an angle $\theta$ about the $z$ axis, $L = a/2\sin(\theta/2)$ the moiré lattice constant and $\boldsymbol{u} = \boldsymbol{u}_1 - \boldsymbol{u}_2$ the acoustic displacement field due to atomic reconstruction where the subscript denotes the layer. The latter reconstructs the rigid moiré pattern leading to domain-wall formation at sufficiently small twist angles. This is illustrated in Fig. S5. The moiré lattice is then defined by

$$\boldsymbol{\phi}(\boldsymbol{r}+\boldsymbol{L}) = \boldsymbol{\phi}(\boldsymbol{r}) + \boldsymbol{a}, \tag{S16}$$

with $\boldsymbol{L} = (L/a)\boldsymbol{a}\times\hat{z}$ a moiré lattice vector and $\boldsymbol{a}$ a monolayer lattice vector.

In the local-stacking approximation, we replace the constant stacking configuration $\boldsymbol{\phi}$ in the Hamiltonian by Eq. (S15) [1] including the effect of lattice relaxation:

$$H_Q(\boldsymbol{k},\boldsymbol{\phi}) \to H_Q[-i\nabla, \boldsymbol{\phi}(\boldsymbol{r})]. \tag{S17}$$

Note that this does not take into account the effect of strain. For the $\Gamma_v$ valley, we can write the resulting moiré continuum theory as $H_\Gamma = \sum_{s=\uparrow,\downarrow}\int d^2\boldsymbol{r}\,\psi_s^\dagger(\boldsymbol{r})\mathcal{H}_\Gamma\psi_s(\boldsymbol{r})$ with

$$\mathcal{H}_\Gamma = \begin{bmatrix} -\frac{\hbar^2\nabla^2}{2m_\Gamma} + \epsilon(\boldsymbol{r}) + \frac{V_z}{2} & t(\boldsymbol{r}) \\ t(\boldsymbol{r}) & -\frac{\hbar^2\nabla^2}{2m_\Gamma} + \epsilon(-\boldsymbol{r}) - \frac{V_z}{2}\end{bmatrix}, \tag{S18}$$

where $\psi_s = (\psi_{s1}, \psi_{s2})^\top$ are fermion field operators in layer space that obey the usual anticommutation relations. Here we define the moiré potentials $\epsilon(\boldsymbol{r}) = \epsilon[\boldsymbol{\phi}(\boldsymbol{r})]$ and $t(\boldsymbol{r}) = t[\boldsymbol{\phi}(\boldsymbol{r})]$ as

$$\boldsymbol{b}\cdot\boldsymbol{\phi}(\boldsymbol{r}) = \boldsymbol{g}\cdot\boldsymbol{r} + \boldsymbol{b}\cdot\boldsymbol{u}(\boldsymbol{r}), \tag{S19}$$

with moiré reciprocal vectors $\boldsymbol{g} = (a/L)\boldsymbol{b}\times\hat{z}$. We also include an interlayer bias $V_z$ which corresponds to an electric displacement that is always present in a single-gate device for STM experiments [2].

The moiré bands are then obtained by making use of the fact that the Hamiltonian is moiré periodic. Using Bloch's theorem, we have the *ansatz*

$$\psi_s(\boldsymbol{r}) = \frac{1}{\sqrt{A}}\sum_{\boldsymbol{k}\in\text{MBZ}}\sum_{\boldsymbol{g}} e^{i(\boldsymbol{k}+\boldsymbol{g})\cdot\boldsymbol{r}} c_{s,\boldsymbol{k}+\boldsymbol{g}}, \tag{S20}$$

with $A$ the system size. Here $\boldsymbol{k}$ is restricted to the moiré Brillouin zone (MBZ) and $c_{s,\boldsymbol{k}+\boldsymbol{g}}$ destroys an electron with spin $s$ and momentum $\boldsymbol{k}+\boldsymbol{g}$. In momentum space, the Hamiltonian then becomes

$$H_\Gamma = \sum_{\boldsymbol{k},s}\sum_{\boldsymbol{g},\boldsymbol{g}} c_{s,\boldsymbol{k}+\boldsymbol{g}}^\dagger \begin{bmatrix} \frac{\hbar^2}{2m_\Gamma}(\boldsymbol{k}+\boldsymbol{g})^2\delta_{\boldsymbol{g},\boldsymbol{g}'} + \epsilon_{\boldsymbol{g}-\boldsymbol{g}'} & t_{\boldsymbol{g}-\boldsymbol{g}'} \\ t_{\boldsymbol{g}-\boldsymbol{g}'} & \frac{\hbar^2}{2m_\Gamma}(\boldsymbol{k}+\boldsymbol{g})^2\delta_{\boldsymbol{g},\boldsymbol{g}'} + \epsilon^*_{\boldsymbol{g}-\boldsymbol{g}'}\end{bmatrix} c_{s,\boldsymbol{k}+\boldsymbol{g}'}, \tag{S21}$$

which describes Bragg scattering processes mediated by the moiré potentials that result in the formation of moiré bands. Here we defined the Fourier transform

$$f_{\boldsymbol{g}} = \frac{1}{A_{\mathrm{m}}} \int_{\text{moiré cell}} d^2\boldsymbol{r}\, f(\boldsymbol{r}) e^{-i\boldsymbol{g}\cdot\boldsymbol{r}}, \tag{S22}$$

with $\boldsymbol{g}$ a moiré reciprocal vector. Here, we used that $\boldsymbol{k}+\boldsymbol{g}$ with $\boldsymbol{k} \in$ MBZ is a unique momentum decomposition and $\int d^2\boldsymbol{r} = \sum_{\boldsymbol{R}} \int_{\text{cell}} d^2\boldsymbol{r}$ with $\sum_{\boldsymbol{R}} e^{i\boldsymbol{k}\cdot\boldsymbol{R}} = N\delta_{\boldsymbol{k}\boldsymbol{0}}$ with $N$ the number of moiré cells. In practice, we diagonalize the Bloch Hamiltonian obtained from Eq. by limiting the number of moiré reciprocal vectors until the moiré bands in the first MBZ are converged.

*Symmetries*

The symmetries of the $\Gamma_v$ moiré system are time-reversal symmetry, the translational symmetry of the moiré, and the moiré point group $D_3 = \langle \mathcal{C}_{3z}, \mathcal{C}_{2y} \rangle$. The latter two yield the wallpaper group $p3m1$. The action of these symmetries on the field operators is chosen as

$$\begin{aligned} \mathcal{T}\psi_s(\boldsymbol{r})\mathcal{T}^{-1} &= \psi_{-s}(\boldsymbol{r}), \\ \mathcal{C}_{2y}\psi_s(x,y)\mathcal{C}_{2y}^{-1} &= \psi_s(-x,y), \\ \mathcal{C}_{3z}\psi_s(\boldsymbol{r})\mathcal{C}_{3z}^{-1} &= \psi_s(\mathcal{C}_{3z}\boldsymbol{r}), \end{aligned} \tag{S23}$$

with $\mathcal{T} i \mathcal{T}^{-1} = -i$. By definition a symmetry requires $[H, \mathcal{S}] = 0$. Hence, time-reversal symmetry implies that all potentials are real. And after a change of integration variables, we find that $\mathcal{C}_{2y}$ symmetry implies

$$\begin{aligned} \epsilon_1(x,y) = \epsilon_2(-x,y) &= \epsilon(x,y), \\ t(x,y) &= t(-x,y), \end{aligned} \tag{S24}$$

for the intralayer moiré potentials and interlayer moiré tunneling. Similarly, threefold rotation symmetry yields

$$\epsilon(\boldsymbol{r}) = \epsilon(\mathcal{C}_{3z}\boldsymbol{r}), \quad t(\boldsymbol{r}) = t(\mathcal{C}_{3z}\boldsymbol{r}). \tag{S25}$$

Moreover, in the local-stacking approximation the theory has an additional model symmetry

$$\mathcal{P}\psi_s(\boldsymbol{r})\mathcal{P}^{-1} = \sigma_x \psi_s(-\boldsymbol{r}), \tag{S26}$$

which is already incorporated in Eq. (S18) and gives

$$\epsilon_1(\boldsymbol{r}) = \epsilon_2(-\boldsymbol{r}), \qquad t(\boldsymbol{r}) = t(-\boldsymbol{r}). \tag{S27}$$

Combining this approximate symmetry with the symmetries of the moiré, the wallpaper group is enhanced to $p6m$ with point group $D_{3d} \cong D_3 \times C_3$. We find

$$\epsilon(x,y) = \epsilon(x,-y), \quad t(x,y) = t(x,-y) = t(-x,y). \tag{S28}$$

Restricting to the first moiré star gives

$$\begin{aligned} \epsilon(\boldsymbol{r}) &= 2V_1 \sum_{i=1}^{3} \cos\left(\boldsymbol{g}_i\cdot\boldsymbol{r} + \psi_1\right), \\ t(\boldsymbol{r}) &= w_0 + 2w_1 \sum_{i=1}^{3} \cos(\boldsymbol{g}_i\cdot\boldsymbol{r}), \end{aligned} \tag{S29}$$

which automatically satisfies the effective inversion symmetry $\mathcal{P}$ which sends $\boldsymbol{r} \mapsto -\boldsymbol{r}$ and flips the layers. In order to break $\mathcal{P}$ one needs to go to the second moiré star and include terms beyond the local-stacking approximation.

Because we are working in the local-stacking approximation, our model will always have an effective inversion symmetry in the absence of symmetry-breaking terms, even if we take into account lattice relaxation. In combination with time-reversal symmetry, this locally protects band crossings in momentum space which can be assigned a fixed chirality. The simplest way to break $\mathcal{P}$ within the local-stacking approximation is the application of an interlayer bias $(V_z/2)\sigma_z$.

| $\lambda$ | $\mu$ | $\sigma$ | $\mathcal{V}_1$ | $\mathcal{V}_2$ | $\mathcal{V}_3$ | $\mathcal{V}_{4,5}$ | $c_1 = \mathcal{V}_1/\mu$ |
|---|---|---|---|---|---|---|---|
| 26437 | 27976 | 0.321 | 10.616 | −2.165 | −0.797 | 0.325 | $3.79 \times 10^{-4}$ |

TABLE S2. Two-dimensional Lamé parameters $\lambda$ and $\mu$, Poisson ration $\sigma = 1/(1 + 2\mu/\lambda)$, and Fourier coefficients of the adhesion potential $\mathcal{V}_n$ of the $n$th reciprocal star (ordered by increasing $|\boldsymbol{b}|$) in units of meV per monolayer unit cell. We also give the dimensionless relaxation parameter $c_1 = \mathcal{V}_1/\mu$. Calculated with DFT for 2H $MoS_2$.

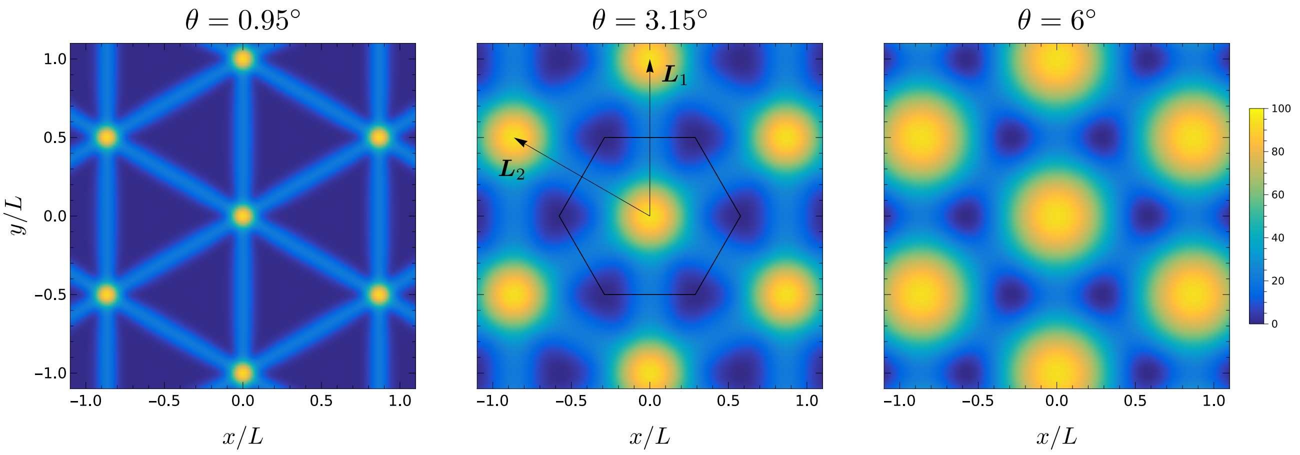


FIG. S5. Adhesion potential $\mathcal{V}[\boldsymbol{\phi}(\boldsymbol{r})]$ in real space in units of meV per monolayer unit cell relative to the lowest-energy configuration for the ground state configuration of aligned twisted bilayer $MoS_2$. Computed with continuum elasticity using the parameters from Table S2. Shown here for three twist angles as indicated.

## S4. LATTICE RELAXATION

We model the atomic reconstruction of the moiré pattern with continuum elasticity [3–6]. In moiré materials, structural reconstruction is driven by a competition between intralayer elastic energy, which prefers the rigid configuration, and interlayer adhesion energy, which favors expanding regions of favorable stacking configurations. We obtained the adhesion potential $\mathcal{V}(\boldsymbol{\phi})$ using the same DFT calculations that were used to obtain the effective electronic Hamiltonian. Here the adhesion potential is defined as the total energy of the bilayer system at charge neutrality minus the energy of two decoupled monolayers. Note that shifting one layer by a monolayer lattice vector $\boldsymbol{a}$ does not change the layer stacking, such that $\mathcal{V}(\boldsymbol{\phi} + \boldsymbol{a}) = \mathcal{V}(\boldsymbol{\phi})$. Furthermore, in our case the adhesion potential has $C_{6v}$ symmetry with respect to $\boldsymbol{\phi} = (\phi_x, \phi_y)$. Taking these symmetries into account,

$$\begin{aligned}\mathcal{V}(\boldsymbol{\phi}) = \mathcal{V}_0 + 2\mathcal{V}_1 \sum_{n=1}^{3} \cos\left(\mathcal{C}_{3z}^n \boldsymbol{b}_1 \cdot \boldsymbol{\phi}\right) \\ + 2\mathcal{V}_2 \sum_{n=1}^{3} \cos\left[\mathcal{C}_{3z}^n (\boldsymbol{b}_1 - \boldsymbol{b}_2) \cdot \boldsymbol{\phi}\right] \\ + 2\mathcal{V}_3 \sum_{n=1}^{3} \cos\left(2\mathcal{C}_{3z}^n \boldsymbol{b}_1 \cdot \boldsymbol{\phi}\right) \\ + \cdots,\end{aligned} \tag{S30}$$

where $\boldsymbol{b}_1 = 4\pi\hat{y}/\sqrt{3}$ and $\boldsymbol{b}_2 = \mathcal{C}_{3z}\boldsymbol{b}_1$. In the following, we set $\mathcal{V}_0 = 0$ as it amounts to a global energy shift independent on the stacking configuration which does not affect the relaxation physics. We restrict ourselves to stacking configurations that are not related by symmetry. Eq. (S30) was fit to the total energy of total of commensurate bilayers, calculated using DFT (see Methods section of the main text). In particular, we consider 37 stacking configurations that are not related by symmetry on a triangular grid (see Fig. S4), which is compatible with the $C_{6v}$ symmetry of the adhesion potential. We then obtain the Fourier coefficients of $\mathcal{V}(\boldsymbol{\phi})$ by performing a linear interpolation and numerically computing

$$\mathcal{V}_{\boldsymbol{b}} = \frac{1}{A_c} \int_{\text{cell}} d^2\boldsymbol{\phi}\, e^{-i\boldsymbol{b}\cdot\boldsymbol{\phi}} \mathcal{V}(\boldsymbol{\phi}), \tag{S31}$$

with $A_c = \sqrt{3}a^2/2$. The coefficients are given in Table S2 together with the elastic constants. The latter are obtained by computing the energy of a 2H $MoS_2$ monolayer subject to constant strain, and performing a fit to continuum elasticity [5]:

$$\mathcal{F}_{\text{elas}}[\boldsymbol{u}] = \frac{1}{2A_c}\int_{\text{cell}} d^2\boldsymbol{r}\left\{(\lambda+\mu)\left(u_{xx}+u_{yy}\right)^2 + \mu\left[\left(u_{xx}-u_{yy}\right)^2 + 4u_{xy}^2\right]\right\}, \tag{S32}$$

where $\lambda$ and $\mu$ are the two-dimensional Lamé parameters, or alternatively, $\lambda+\mu$ is the bulk modulus and $\mu$ is the shear modulus. Here

$$u_{ij}(\boldsymbol{r}) = \frac{1}{2}\left(\frac{\partial u_j}{\partial r_i} + \frac{\partial u_i}{\partial r_j}\right), \tag{S33}$$

is the strain tensor with $\boldsymbol{u}$ the in-plane displacement field of a single layer (note that this differs from the previous notation). Here, we neglected quadratic corrections from out-of-plane displacements.

To model atomic reconstruction in a moiré superlattice, we use continuum elasticity, which is a good approximation for small twist angles where $L \gg a$ and the local stacking varies slowly compared to the interatomic scale. We minimize the total strain and adhesion energy of the twisted bilayer with respect to the stacking configuration $\boldsymbol{\phi}(\boldsymbol{r})$ under periodic boundary conditions in the moiré supercell. We have

$$\begin{aligned}\mathcal{F} &= \mathcal{F}_{\text{elas}}[\boldsymbol{u}_1] + \mathcal{F}_{\text{elas}}[\boldsymbol{u}_2] + \mathcal{F}_{\text{adh}}[\boldsymbol{\phi}] \\ &= \mathcal{F}_{\text{elas}}\left[\frac{\boldsymbol{u}_1+\boldsymbol{u}_2}{2}\right] + \mathcal{F}_{\text{elas}}\left[\frac{\boldsymbol{u}_1-\boldsymbol{u}_2}{2}\right] \\ &\quad + \mathcal{F}_{\text{adh}}[\boldsymbol{\phi}],\end{aligned} \tag{S34}$$

where the elastic energy of the bilayer system is obtained by summing both layer contributions $\boldsymbol{u}_1$ and $\boldsymbol{u}_2$. Moreover, in the absence of out-of-plane strain contributions, the elastic term decouples into functionals that only depend on $\boldsymbol{u}_1+\boldsymbol{u}_2$ and $\boldsymbol{u}_1-\boldsymbol{u}_2$. Since the interlayer energy depends only on $\boldsymbol{u}_1-\boldsymbol{u}_2$ we can ignore the contribution from the layer symmetric part. Up to constants and boundary terms that vanish for periodic boundary conditions, the elastic and adhesion contributions can be written as:

$$\begin{aligned}\mathcal{F}_{\text{elas}}[\boldsymbol{\phi}(\boldsymbol{r})/2] &= \frac{1}{A_m}\int_{\text{moiré cell}} d^2\boldsymbol{r}\left[\frac{\lambda}{4}\left(\partial_i\phi_i\right)^2 + \frac{\mu}{8}\left(\partial_i\phi_j + \partial_j\phi_i\right)^2\right], \\ \mathcal{F}_{\text{adh}}[\boldsymbol{\phi}(\boldsymbol{r})] &= \frac{1}{A_m}\int_{\text{moiré cell}} d^2\boldsymbol{r}\,\mathcal{V}[\boldsymbol{\phi}(\boldsymbol{r})],\end{aligned} \tag{S35}$$

with $A_m = \sqrt{3}L^2/2$ and where summation over repeated indices is implied in the first line.

Since we have assumed that the relative atomic displacement field $\boldsymbol{u}(\boldsymbol{r}) = \boldsymbol{u}_1(\boldsymbol{r}) - \boldsymbol{u}_2(\boldsymbol{r})$ has the periodicity of the moiré lattice, we can write $\boldsymbol{u}(\boldsymbol{r}) = \sum_{\boldsymbol{g}} \boldsymbol{u}_{\boldsymbol{g}} e^{i\boldsymbol{g}\cdot\boldsymbol{r}}$ where $\boldsymbol{g}$ are moiré reciprocal vectors. More details on this approach and its numerical implementation can be found in Ref. [6]. The resulting ground state configurations are illustrated in Fig. S5 for three twist angles corresponding to strong, intermediate and weak reconstruction. We note that our theory for lattice relaxation applies to any moiré system with identical stacking symmetries, including twisted bilayer graphene (tBG) [3] and other moiré systems comprised of TMDs, including twisted bilayers of 2H monolayers near 0° (such as t$MoS_2$) and 1T near 60°. The important dimensionless parameter of this theory is given by $c_1/\theta^2$ with $c_1 = \mathcal{V}_1/\mu$ [6? ]. Hence, the same structural moiré reconstruction is expected as compared to tBG for

$$\frac{\theta_{\text{tMoS}_2}}{\theta_{\text{tBG}}} = \sqrt{\frac{c_{1,\text{tMoS}_2}}{c_{1,\text{tBG}}}} \approx 3, \tag{S36}$$

where the value of $c_1$ for t$MoS_2$ is listed in Table S2 and $c_{1,\text{tBG}} \approx 4.5 \times 10^{-5}$ [? ].

In Fig. S7 we show the relaxed $\Gamma_v$-valley and $K_c/K_c'$ moiré potentials $\epsilon[\boldsymbol{\phi}(\boldsymbol{r})]$ and $t[\boldsymbol{\phi}(\boldsymbol{r})]$ for $\theta = 0.95°$ calculated using the parameters from Table S1 and the atomic displacement field obtained from continuum elasticity. We also show the nearly rigid (unrelaxed) moiré potentials for $\theta = 6°$ for comparison.

## S5. MOIRÉ BAND STRUCTURE

The moiré bands are obtained by writing down a Bloch *ansatz* for the moiré continuum theory in terms of a plane-wave expansion. Below, we briefly discuss our results for the moiré bands near both the valence band maximum ($\Gamma_v$) and the conduction band minimum ($K_c/K_c'$).

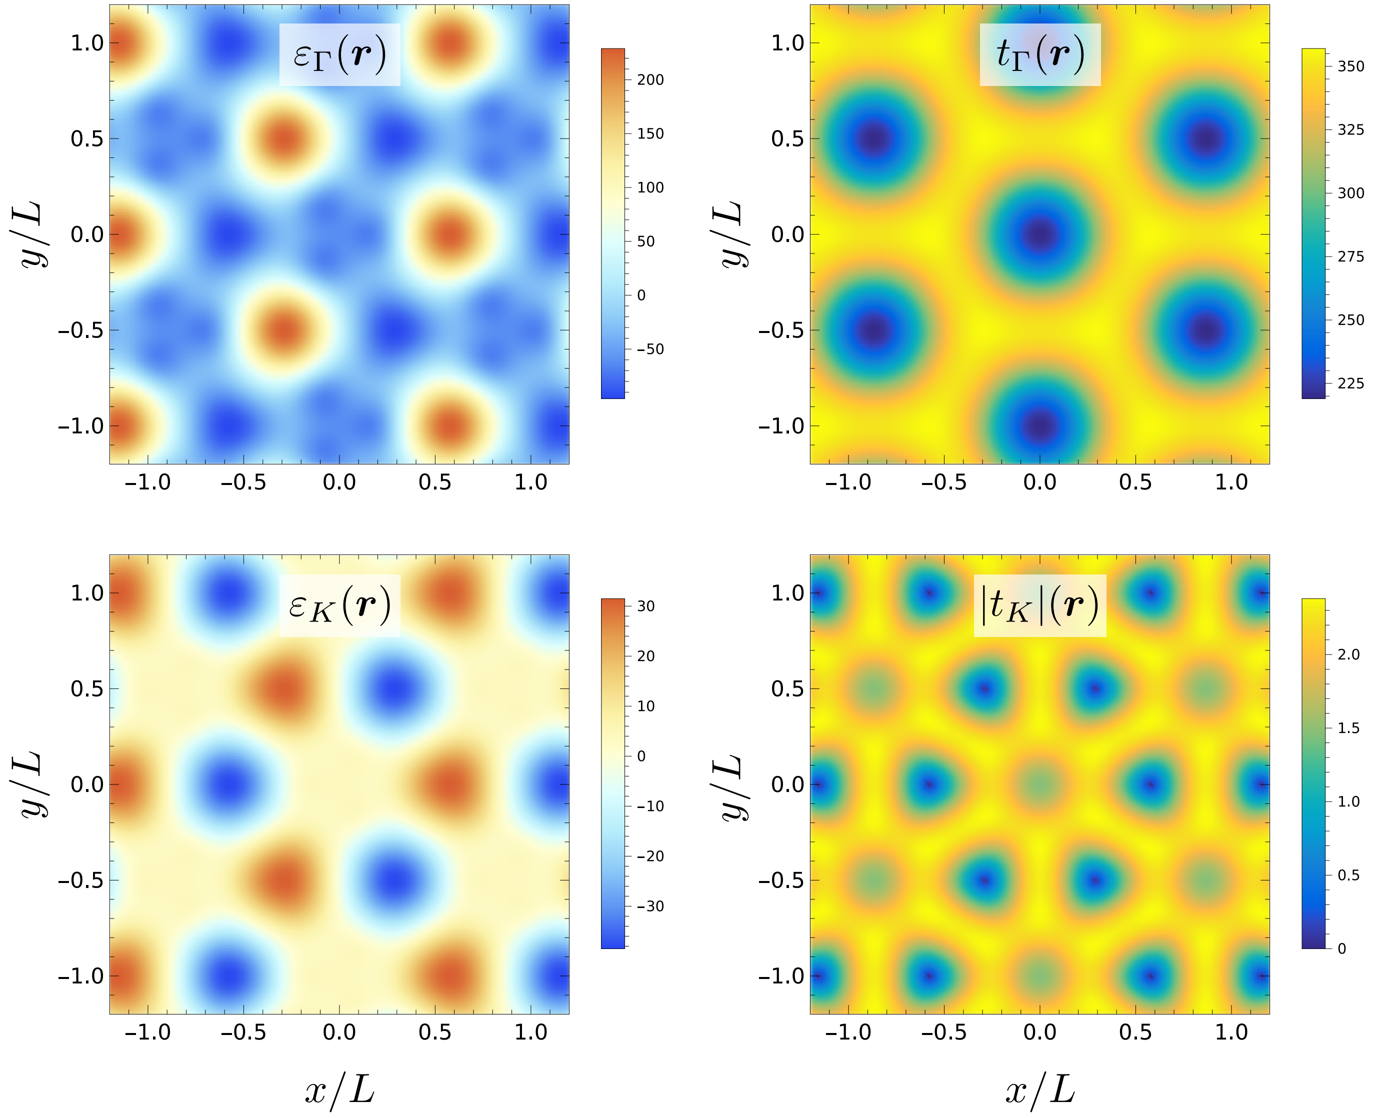


FIG. S6. Relaxed moiré intralayer potential $\varepsilon(\boldsymbol{r})$ and interlayer tunneling $t(\boldsymbol{r})$ for aligned tMoS$_2$ with $\theta = 6^\circ$ at the $\Gamma_v$ (top panel) and $K_c/K_c'$ (bottom panel) point as indicated.

## A. $\Gamma_v$ valley

*Relaxed moiré bands*

We show the $\Gamma_v$-valley moiré bands for several twist angles in Fig. S8 with and without moiré reconstruction. When relaxation is relatively weak, the qualitative features of the moiré bands remain. This is the case around $3.15^\circ$ shown on rightmost panel of Fig. S8. However, as the twist angle decreases the reconstruction of the moiré pattern completely changes the low-energy moiré bands. This is illustrated for $2^\circ$ and $0.95^\circ$, which is the case corresponding to the experiment. For the latter, only the topmost two rigid moiré bands are visible in the plot. To further illustrate this, we also show the bandwidth of the topmost manifold of two moiré bands of the $\Gamma_v$ valley for the rigid and relaxed case in Fig. S8(a) as a function of twist angle, together with the gap between the second and third moiré band in S8(b). In general, we find that the bandwidth increases when relaxation is included. For the other manifolds of moiré bands, we find that only the $p$-wave manifold of four bands survives, while the effective kagome lattice discussed in Ref. [7].

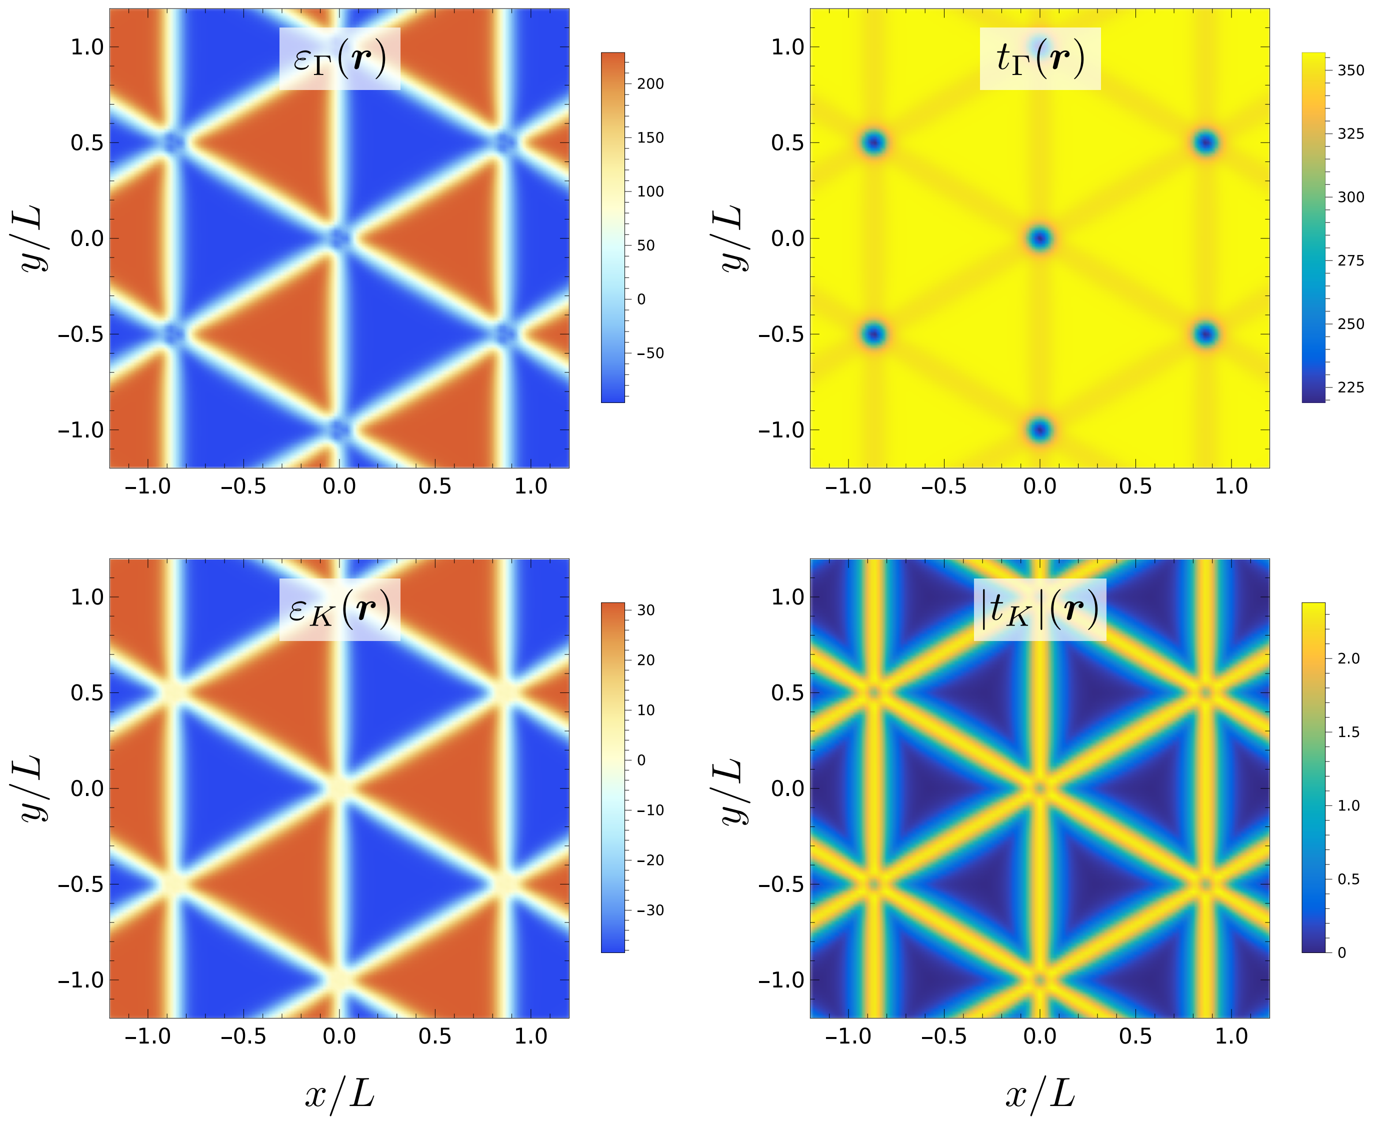


FIG. S7. Relaxed moiré intralayer potential $\varepsilon(\boldsymbol{r})$ and interlayer tunneling $t(\boldsymbol{r})$ for aligned tMoS$_2$ with $\theta = 0.95°$ at the $\Gamma_v$ (top panel) and $K_c/K_c'$ (bottom panel) point as indicated.

*Effective honeycomb lattice*

The top two (spin degenerate) $\Gamma_v$ moiré bands correspond to an effective honeycomb lattice [7**?** ]. Here the sublattices correspond to $s$-like orbitals that originate from the *intralayer* moiré potential which gives rise to an array of triangular potential well, see Fig. S7. These orbitals are centered at the MX and XM stacking centers in the top and bottom layer, respectively, depending on the sign of the twist angle. The *interlayer* moiré tunneling couples the two orbitals giving rise to an effective nearest-neighbor hopping. Hence the top two moiré bands form an artificial honeycomb lattice of holes whose sublattices are given by the layer degree of freedom. We note that the combination $\mathcal{PT}$ of the effective inversion symmetry $\mathcal{P}(\boldsymbol{r} \mapsto -\boldsymbol{r}, \sigma_x)$ that is inherited from the untwisted bilayers in the local-stacking approximation, and time-reversal symmetry $\mathcal{T}$ locally protects the crossings at $\kappa$ and $\kappa'$ in the moiré Brillouin zone.

However, an interlayer bias $V_z$ breaks $\mathcal{P}$ symmetry and opens a gap, giving rise to two layer-polarized, and therefore MX/XM polarized bands. This is illustrated in Fig. S10. Here, the layer polarization of the topmost bands is approximately 0.5 such that 75 % of the states are localized in one layer. Full layer polarization requires $V_z \gtrsim w_0$ the interlayer tunneling energy scale. When $V_z$ becomes large enough, the topmost states display the same degeneracy $(1, 2, 1, 2, 2, \ldots)$ and approximate energy ratios of a particle in an equilateral triangular infinite well [**?** ]. This is because when $V_z$ is large, one can integrate out the other layer resulting effectively in a triangular array of quantum

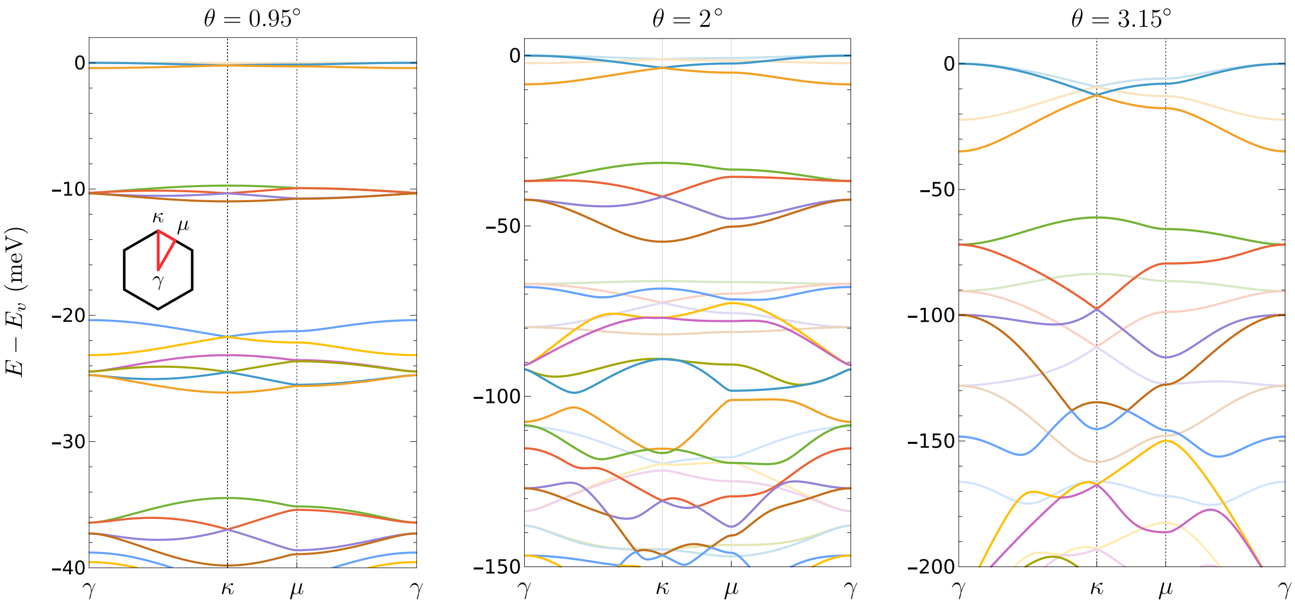


FIG. S8. $\Gamma_v$-valley moiré bands for twist angles corresponding to intermediate ($\theta = 3.15°$ and $2°$) and strong ($\theta = 0.95°$) moiré reconstruction. The rigid and relaxed moiré bands are shown in light and dark colors, respectively. For $\theta = 0.95°$ the only the top rigid moiré band is visible in the energy range shown.

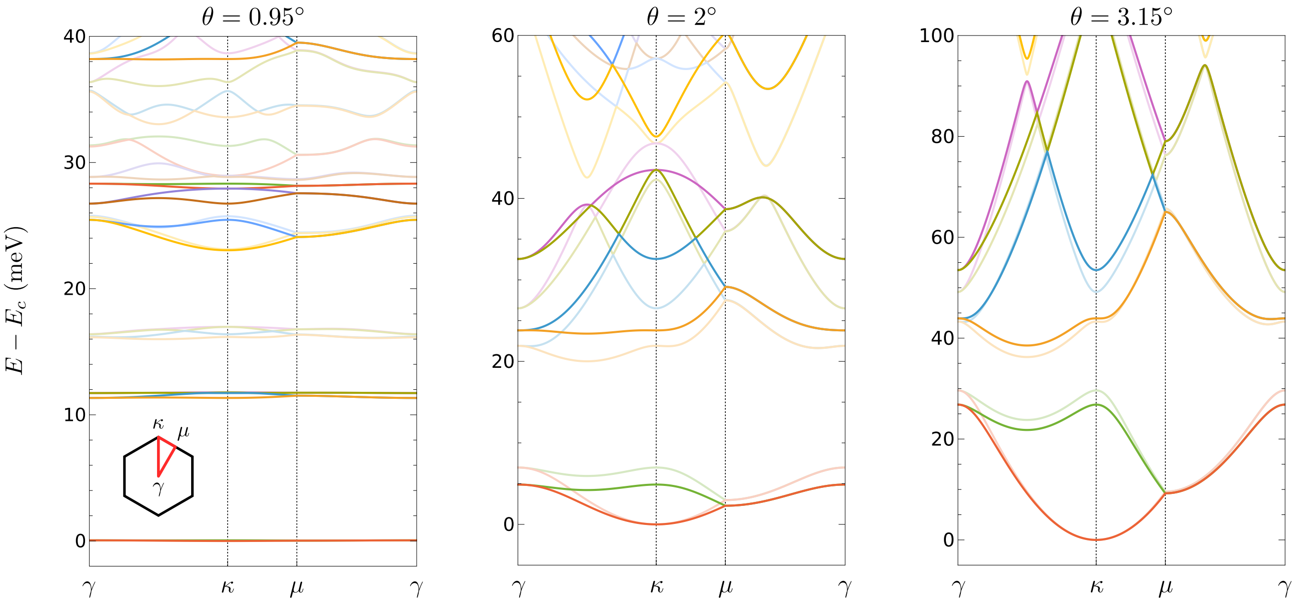


FIG. S9. $K_c/K_c'$-valley moiré bands for twist angles corresponding to intermediate ($\theta = 3.15°$ and $2°$) and strong ($\theta = 0.95°$) moiré reconstruction. The rigid and relaxed moiré bands are shown in light and dark colors, respectively.

dots where the potential is effectively given by the intralayer moiré potential shown in Fig. S7.

### B. $K_c/K_c'$ valley

At the bottom of the conduction band, the moiré effect is much weaker, see Figs. S6 and S7. We find that interlayer tunneling is weak and the layers are almost decoupled, which is further suppressed by the reconstruction of the moiré patter. This is because interlayer tunneling is symmetry-forbidden for $MX/XM$ stacking. Thus, the moiré bands are essentially layer polarized, and the effect of the interlayer bias is strong, in contrast with the $\Gamma_v$ moiré bands where the layers are strongly hybridized. Nevertheless, the moiré still imprints an effective intralayer potential at $K_c/K_c'$

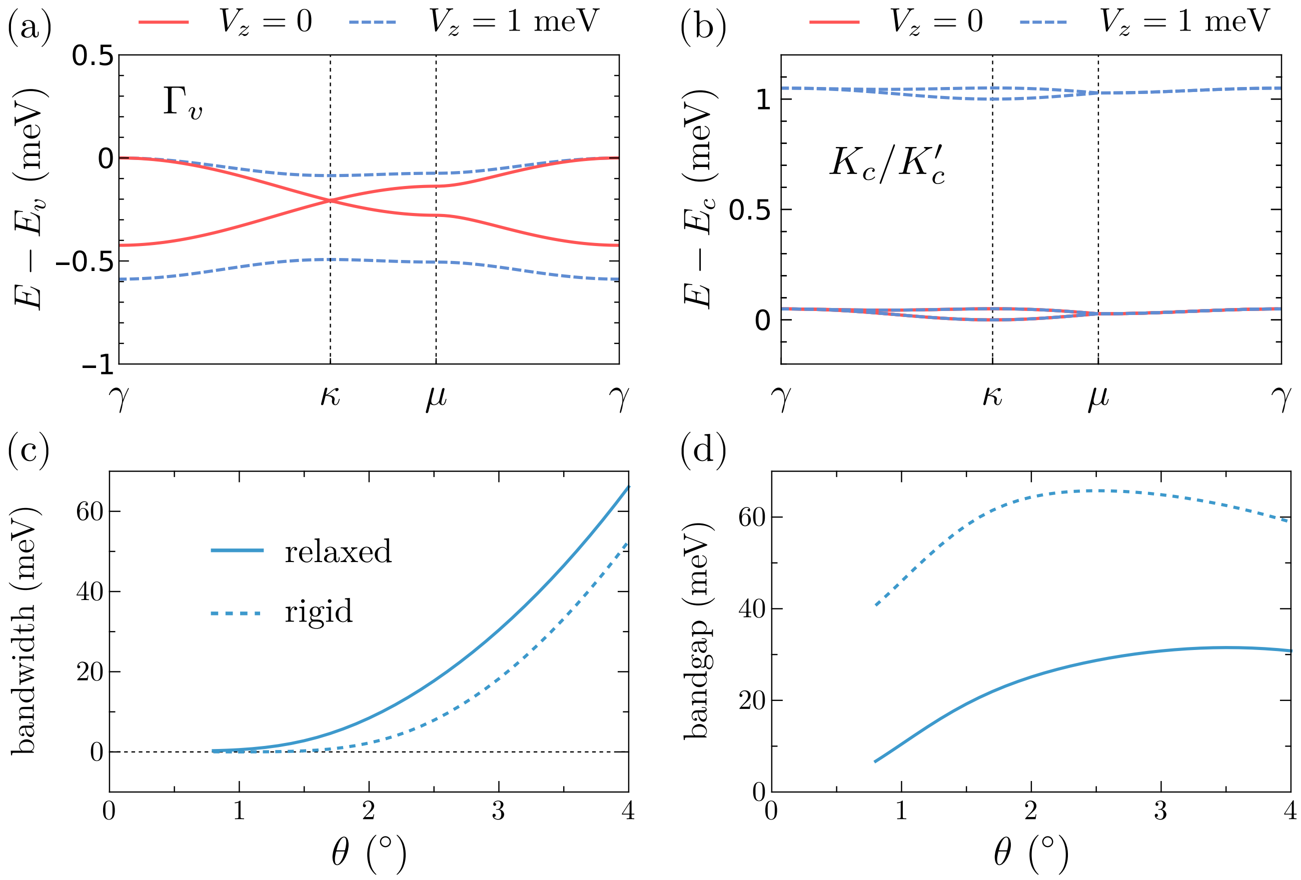


FIG. S10. $\Gamma_v$-valley moiré bands for twist angle $\theta = 0.95°$ including the effect of lattice relaxation for several values of the interlayer bias $V_z$ as indicated. The layer polarization $\langle \sigma_z \rangle$ of each state is indicated by the color. Note that between $V_z = 20$ meV and $V_z = 30$ meV the second band interchanges with the degenerate third and fourth bands.

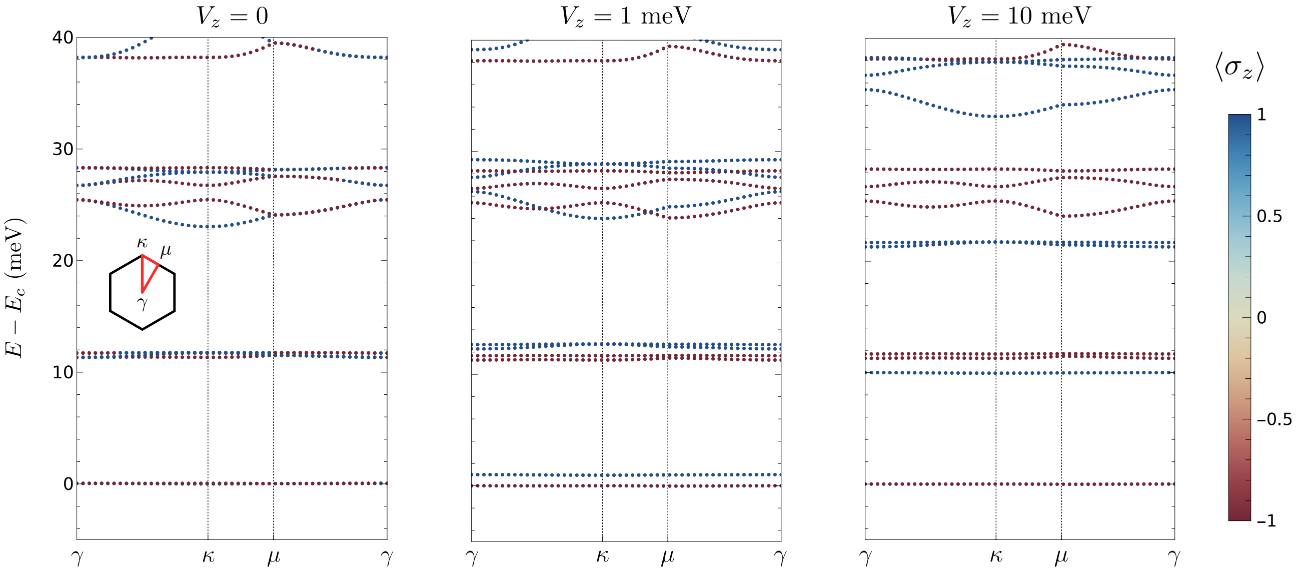


FIG. S11. $K_c/K_c'$-valley moiré bands for twist angle $\theta = 0.95°$ including the effect of lattice relaxation for several values of the interlayer bias $V_z$ as indicated. The layer polarization $\langle \sigma_z \rangle$ of each state is indicated by the color.

resulting in moiré bands, shown in Fig. S9. Now the moiré bands are further flattened by lattice reconstruction as this increases electron localization resulting in a periodic array of weakly coupled triangular quantum dots in each layer. We further show in Fig. **??** that the interlayer bias, unlike the strongly layer-hybridized $\Gamma_v$ moiré bands, simply rigidly shifts the bands, as expected for decoupled layers.

## S6. LOCAL DENSITY OF STATES

To compare our theory to the STM measurements described in the main text, we compute the local density of states (LDOS)

$$\rho(\boldsymbol{r}, E) = \sum_{n,\boldsymbol{k}} \delta(E - E_{n\boldsymbol{k}}) |\psi_{n,\boldsymbol{k}}(\boldsymbol{r})|^2, \tag{S37}$$

where $n$ is a band index (including spin, as well as valley for $K_c/K_c'$). Here the total wave function squared includes a sum over both layers and reciprocal moiré vectors of the plane-wave expansion.

To account for disorder, we introduce a phenomenological broadening parameter $\gamma$ and replace the delta function with a Lorentzian:

$$\delta(E - E_{n\boldsymbol{k}}) \to \frac{1}{\pi} \frac{\gamma}{(E - E_{n\boldsymbol{k}})^2 + \gamma^2}, \tag{S38}$$

with a full width at half maximum given by $2\gamma$.

We are particularly interested in the LDOS at the high-symmetry stacking centers: MM, XM, MX, and DW. In our coordinates, we take

$$\boldsymbol{r}_{\mathrm{MM}} = (0, 0), \tag{S39}$$

$$\boldsymbol{r}_{\mathrm{XM}} = -\boldsymbol{r}_{\mathrm{MX}} = (L/\sqrt{3}, 0), \tag{S40}$$

$$\boldsymbol{r}_{\mathrm{DW}} = (0, L/2), \tag{S41}$$

with $L = a/[2\sin(\theta/2)]$ the moiré period.

The calculated LDOS is shown in Fig. S12 for the $\Gamma_v$ moiré bands for several values of the interlayer energy bias $V_z$ and the broadening parameter $\gamma$. We find that a value of $V_z = 20$ meV and $\gamma = 10$ meV can qualitatively reproduce the onset shift between XM and MX observed in the experiment. Hence, the onset shift is effectively a measurement of the moiré gap between the first two layer-projected moiré bands, see Fig. S10. We note that the estimated charge disorder in the experiment $\delta n$ is almost the same as the density of a single moiré band $n_m = 2/A_m \approx (1^\circ/\theta)^2\, 6.9 \times 10^{11}$ cm$^{-2}$. This is why the experiment cannot resolve any individual moiré bands, and the broadening parameter is on the order of the gap between subsequent moiré bands.

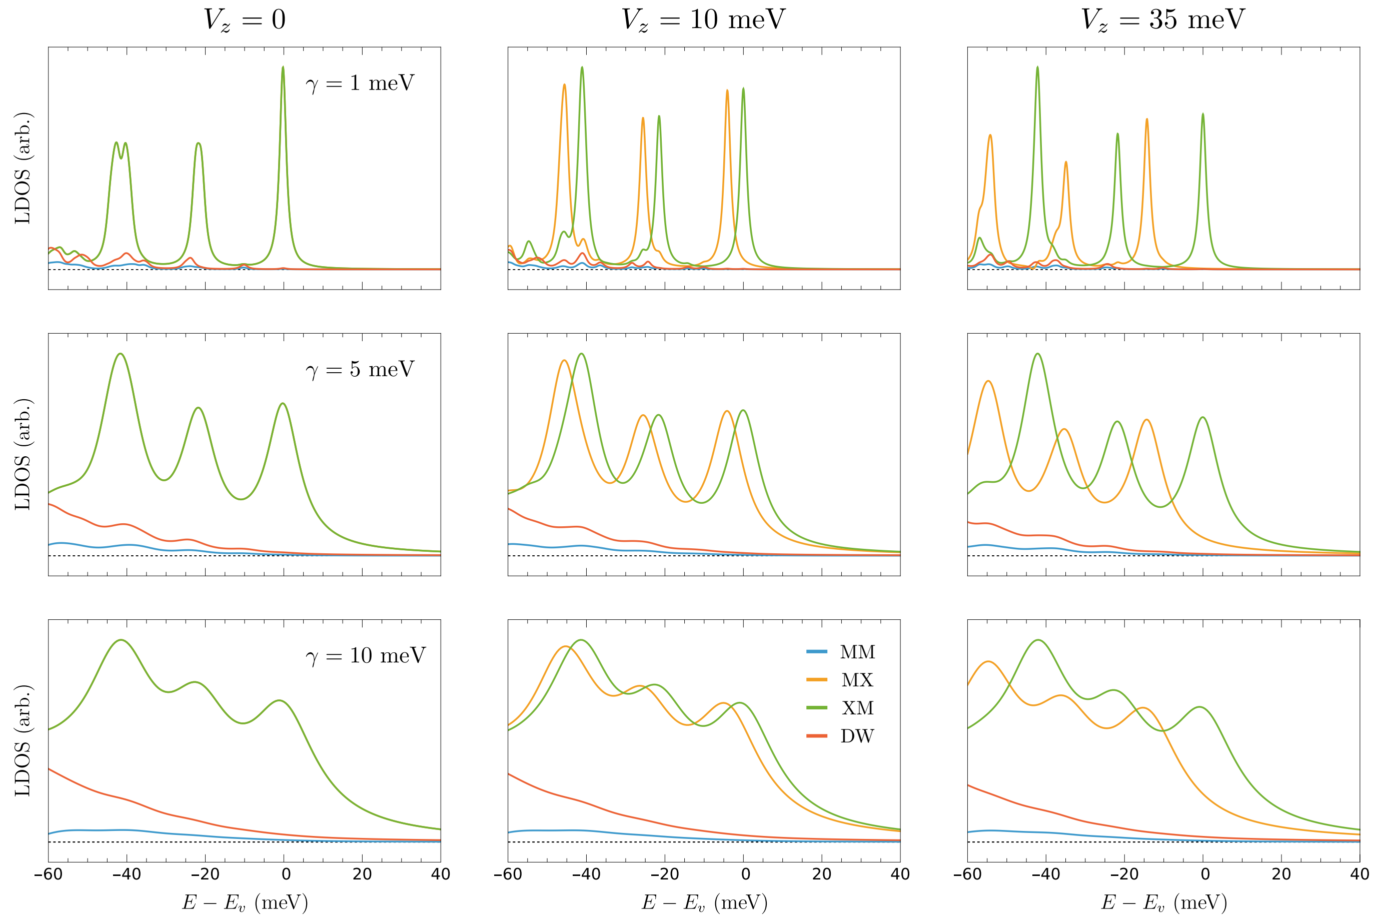


FIG. S12. LDOS at different positions in the moiré cell for the $\Gamma_v$ moiré bands of aligned tb-$MoS_2$ at twist angle $\theta = 0.95°$. We include the effect of lattice relaxation and show several values of the interlayer bias $V_z$ and phenomenological broadening parameter $\gamma$ as indicated.

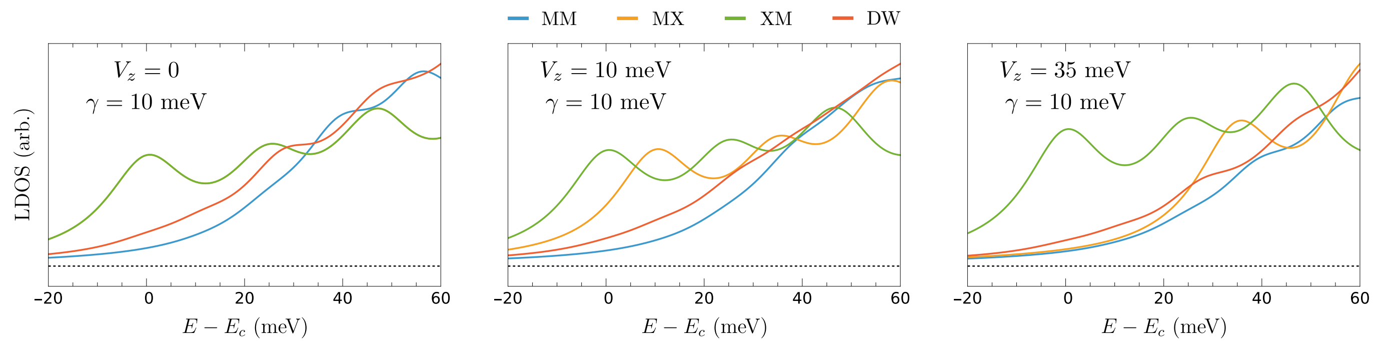


FIG. S13. LDOS at different positions in the moiré cell for the $K_c/K_c'$ moiré bands of aligned tb-$MoS_2$ at twist angle $\theta = 0.95°$. We include the effect of lattice relaxation and show several values of the interlayer bias $V_z$ and take $\gamma = 10$ meV.

[1] J. Jung, A. M. DaSilva, A. H. MacDonald, and S. Adam, Origin of band gaps in graphene on hexagonal boron nitride, Nat. Commun. **6**, 6308 (2015).

[2] A. Garcia-Ruiz and M.-H. Liu, Twisted bilayer $MoS_2$ under electric fields: A system with tunable symmetry, Nano Lett. **24**, 16317 (2024).

[3] N. N. T. Nam and M. Koshino, Lattice relaxation and energy band modulation in twisted bilayer graphene, Phys. Rev. B **96**, 075311 (2017).

[4] S. Carr, D. Massatt, S. B. Torrisi, P. Cazeaux, M. Luskin, and E. Kaxiras, Relaxation and domain formation in incommensurate two-dimensional heterostructures, Phys. Rev. B **98**, 224102 (2018).

[5] D. Bennett, Theory of polar domains in moiré heterostructures, Phys. Rev. B **105**, 235445 (2022).

[6] C. De Beule, G. N. Pallewela, M. M. Al Ezzi, L. Peng, E. J. Mele, and S. Adam, Theory for lattice relaxation in marginal twist moirés (2025).

[7] M. Angeli and A. H. MacDonald, Gamma valley transition metal dichalcogenide moiré bands, Proc. Natl. Acad. Sci. U.S.A. **118**, e2021826118 (2021).
